# Supplementary material for: ObjTables: structured spreadsheets that promote data quality, reuse, and integration
Source: arXiv:2005.05227 source file (2020-08-06)
Supplement: Supplementary file 1 [file Supplementary_information.pdf]

# *ObjTables*: structured spreadsheets that promote data quality, reuse, and integration

# *Supplementary information*

Jonathan R. Karr[1,2*], Wolfram Liebermeister[3], Arthur P. Goldberg[1,2], John A. P. Sekar[1,2] & Bilal Shaikh[1,2]

August 6, 2020

[1]Icahn Institute for Data Science and Genomic Technology, Icahn School of Medicine at Mount Sinai, New York, NY 10029, USA.

[2]Department of Genetics and Genomic Sciences, Icahn School of Medicine at Mount Sinai, New York, NY 10029, USA.

[3]Université Paris-Saclay, INRAE, MaIAGE, 78350, Jouy-en-Josas, France.

*Corresponding author: Jonathan Karr (karr@mssm.edu)

This manuscript describes version 1.0.11 of *ObjTables*.

## Contents


**1 Overview of *ObjTables*** **3**
- 1.1 Design choices: Standalone program for working with enhanced XLSX files . . . . . 3
- 1.2 Develop software tools that complement existing spreadsheet programs . . . . . . . 3
- 1.3 Format for structured, human-readable spreadsheets . . . . . . . . . . . . . . . . . 4
- 1.4 Format for schemas for structured, human-readable spreadsheets . . . . . . . . . . 6
- 1.5 Tools for systematically controlling the quality of data in spreadsheets . . . . . . . 7
- 1.6 Programmatically creating, querying, editing and analyzing spreadsheets . . . . . . 8
- 1.7 Comparing the content of spreadsheets . . . . . . . . . . . . . . . . . . . . . . . 8
- 1.8 Merging and splitting spreadsheets . . . . . . . . . . . . . . . . . . . . . . . . . 8
- 1.9 Revisioning and migrating spreadsheets . . . . . . . . . . . . . . . . . . . . . . . 8
- 1.10 Converting spreadsheets to and from alternative formats . . . . . . . . . . . . . . 9
- 1.11 Visualizing the structure of a spreadsheet . . . . . . . . . . . . . . . . . . . . . . 9
- 1.12 User interfaces . . . . . . . . . . . . . . . . . . . . . . . . . . . . . . . . . . . . 9

**2 Implementation and testing of *ObjTables*** **9**

**3 Case studies of using *ObjTables* to structure, debug, reuse, and compose data** **10**
- 3.1 An integrated kinetic-thermodynamic genome-scale model of *E. coli* metabolism . . 10
- 3.2 Format for composite, multi-algorithmic whole-cell models . . . . . . . . . . . . . . 12

**4 Comparison of *ObjTables* with other tools** **13**
- 4.1 Domain-specific spreadsheet schemas . . . . . . . . . . . . . . . . . . . . . . . . 13
- 4.2 Alternative general-purpose tools for combining spreadsheets with schemas . . . . . 13
- 4.3 Databases and object-relational mapping (ORM) tools . . . . . . . . . . . . . . . . 14
- 4.4 Hybrid database-spreadsheet tools such as DataSpread . . . . . . . . . . . . . . . 14
- 4.5 Data serialization formats such as JSON, XML, and YAML . . . . . . . . . . . . . . 15

**5 Future directions for *ObjTables*** **15**
- 5.1 Additional types of attributes for additional types of data . . . . . . . . . . . . . . 15
- 5.2 Additional layouts to make some datasets easier for humans to read . . . . . . . . . 15
- 5.3 Libraries for additional programming languages . . . . . . . . . . . . . . . . . . . 15
- 5.4 A registry of schemas to facilitate standardization . . . . . . . . . . . . . . . . . . 15
- 5.5 Graphical user interface viewing and edits *ObjTables*-encoded spreadsheets . . . . 16
- 5.6 Community adoption of *ObjTables* as a meta-standard for data . . . . . . . . . . . 16

# 1. Overview of *ObjTables*

The *ObjTables* toolkit includes several interrelated tools for creating, validating, and reusing structured, human-readable spreadsheets. Here, we outline the design rationale for *ObjTables*; the components of the toolkit, including the format for structured, human-readable spreadsheets; the format for schemas and supported data types; software tools for validating, comparing, and pretty-printing spreadsheets; and a Python package for more advanced operations such as analyzing, merging, splitting, revisioning, and migrating spreadsheets. Additional examples, tutorials, and more detailed documentation are available at https://objtables.org.

## 1.1. Design choices: Standalone program for working with enhanced XLSX files

We designed *ObjTables* as a complement to the Office Open Spreadsheet XML format (XLSX; ECMA-376;[1] ISO/IEC 29500[2]) for several reasons.

### 1.1.1. Expand the capabilities of an open file format that researchers already commonly use to share data

To make *ObjTables* an appealing option for supplementary datasets to journal articles, we wanted to base *ObjTables* on a file format that is easy for many researchers to read, and which is already a popular format for supplementary data. Furthermore, we wanted to base *ObjTables* on an open format. This narrowed our choices to the XLSX format and text-based formats such as CSV or TSV. While data serialization formats such as JSON, XML, and YAML provide some of the benefits of *ObjTables*, we did not want to base *ObjTables* on these formats because the GUI tools for these files do not make datasets as easy to read as spreadsheets programs such as Excel.

Although databases and ORMs also provide some of the benefits of *ObjTables*, we did not want to base *ObjTables* on a traditional relational database or a low-code database such as Airtable because we wanted journals to be able to archive datasets as a file, and we wanted readers to be able to use simple tools to read these files. Relational databases are too complex for many researchers, and commercial low-code tools are not designed to export and import datasets to and from files, which is critical for journal archiving. Another reason why we chose to base *ObjTables* on a file format rather than a database is that we wanted *ObjTables* to be compatible with asynchronous collaboration workflows with version control systems such as Git.

As a result, we chose to base *ObjTables* on top of the XLSX format, a popular and open format for spreadsheets.

## 1.2. Develop software tools that complement existing spreadsheet programs

Due to the popularity and significant capabilities of existing spreadsheet programs such as Excel, we wanted to enable users to continue to use their favorite programs on their favorite operating systems as much as possible. In particular, we wanted peer reviewers, editors, and readers of journal articles to be able to read *ObjTables*-encoded spreadsheets with their existing spreadsheet programs rather than have to install an additional program to read a dataset. We also wanted authors to be able to continue to do the majority of their work (e.g., combine data from multiple sources, munge each source, perform calculations, make charts) with their favorite spreadsheet program and only briefly have to use a new program for advanced features such as validation that are not available in programs such as Excel.

We did not want to develop an extension for a spreadsheet program such as Excel or Google Sheets because this would only benefit users of that one program as there is no universal format for extensions. In addition, an extension would only benefit users of specific versions of that program on specific operating systems because the interfaces for extensions change over time. We also did not want to build the *ObjTables* software as an extension of Microsoft Excel or Google Sheets because we wanted researchers to be able to use *ObjTables* with free, open-source tools. We did not want to build the *ObjTables* software as an extension of an open-source spreadsheet tool such as LibreOffice Calc because these tools are much less popular than Excel.

As a result, we chose to develop the *ObjTables* software as a separate, OS-independent program from spreadsheet programs such as Excel. Furthermore, we tried to make the software as accessible as possible by providing it as a web application, command-line program, web service, and Python package.

## 1.3. Format for structured, human-readable spreadsheets

*ObjTables* builds upon the Office Open Spreadsheet XML format (XLSX; ECMA-376;[1] ISO/IEC 29500[2]). To make spreadsheets both machine and human-readable, *ObjTables* incorporates the additional layout conventions and markup syntax described below. These conventions and syntax expand on ideas pioneered by SBtab.[3] As an example, Fig. 1 of the main text illustrates how a dataset of the transcripts and genes of an organism can be encoded into a spreadsheet. More detailed documentation is available at https://objtables.org.

### 1.3.1. Declaring that a spreadsheet is encoded in the *ObjTables* format

To communicate that a spreadsheet uses the *ObjTables* format, *ObjTables* includes an additional worksheet that contains a table of contents for the spreadsheet. The first row of the table of contents worksheet contains a single cell which begins with the markup `!!!ObjTables`. As described below, this row can also contain metadata about the dataset. The other rows of the table of contents worksheet describe and provide hyperlinks to the worksheets which represent the data. *ObjTables* indicates the table of contents worksheet with the title `!!_Table of contents`. As described below, the *ObjTables* software can automatically generate table of contents worksheets for users.

### 1.3.2. Encoding data into spreadsheets

To help users find information in spreadsheets, *ObjTables* encodes each principal class of object in a dataset into a separate worksheet. For example, a dataset of genes and their splice variants would be encoded into two worksheets. *ObjTables* uses two mechanisms to declare that a worksheet represents data. First, data worksheets have titles that begin with the markup `!!`, followed by the name of the class represented by the worksheet. Second, the first row of each data worksheet begins with the markup `!!ObjTables type='Data' class='class-name'`.

*ObjTables* encodes each principal object into a single row in the corresponding worksheet for its class. For example, each gene would be encoded into a row in the 'Genes' worksheet.

*ObjTables* encodes each attribute of each class into a separate column. For example, the id, symbol, chromosome, and 3' and 5' coordinates of genes would be represented by five columns. *ObjTables* encodes the attribute represented by each column into an additional heading row before

the data rows. Each heading begins with the markup `!`, followed by the name of the attribute represented by the column.

To help make datasets easy to read, *ObjTables* can encode related attributes into adjacent columns. *ObjTables* indicates column groups by including an additional heading that spans all of the associated columns in an extra row above the headings for the individual columns. These headings also begin with the markup `!`, followed by the name of the group of attributes. For example, columns that represent the chromosome and 5' and 3' coordinates of genes could be located next to each other and indicated with the joint heading `!Location`.

*ObjTables* utilizes three mechanisms to encode attributes that represent relationships between objects into spreadsheets. First, schemas can define a primary attribute for each class, and *ObjTables* can use their values to reference related objects. An object related via a one-to-one or many-to-one relationship can be encoded into the value of its primary attribute. Objects related via a one-to-many or many-to-many relationship can be encoded into a delimited list of the values of the related objects. To ensure these references can be resolved, schemas must also declare each primary attribute to be unique.

Second, as described above, objects related via a one-to-one or many-to-one relationship to another class can be encoded into a group of adjacent columns, one for each attribute of the related class, within the worksheet which represents the instances of the other class. In some cases, this enables researchers to encode datasets into more human-readable spreadsheets that use a smaller number of worksheets by encoding related information into nearby columns. While similar spreadsheet layouts could be achieved by using flatter schemas with fewer classes, the advantages of the above approach are that it uses bi-level headings to visually group related columns within spreadsheets and that it encapsulates related attributes into separate data structures.

Third, *ObjTables* can use grammars to serialize related objects into a single string-valued column. For example, researchers could use the Nomenclature of Genes, Genetic Markers, Alleles, and Mutations in Mouse and Rat[4] to encode specific alleles such as the spontaneous Mo allele of Atp7a into $\texttt{Atp7a}^{\texttt{Mo}}$ or use the Sequence Variant Nomenclature[5] to encode sequence variants such as the deletion of thymidine at position g.19 of Homo sapiens dystrophin into `NG_012232.1:g.19delT` rather than using additional worksheets to define alleles and sequence variants.

#### 1.3.3. Encoding metadata into spreadsheets

*ObjTables* can encode multiple levels of metadata into spreadsheets. Metadata about an entire dataset can be encoded into the first cell of the table of contents worksheet as pairs of keys and values. For example, the author of a dataset can be captured by the syntax `author='John Doe'`. Similarly, metadata about a class can be encoded into the first cell of the corresponding worksheet. Metadata about an object can be encoded into an additional row above the row that represents the object. Metadata rows contain a single cell that contains a textual comment between the markup delimiters `%/` and `/%`.

#### 1.3.4. Encoding schema documentation into spreadsheets

To best leverage spreadsheet programs such as Microsoft Excel and LibreOffice Calc as editors for *ObjTables* datasets, to the extent permitted by the XLSX format, *ObjTables* encodes the type of each attribute and constraints on its values into validations of the corresponding column. For attributes that represent enumerations and one-to-one and many-to-one relationships, this provides

users dropdown menus for selecting values. This validation can help users quickly find errors, such as an invalid value of an enumerated attribute. Due to the few validations supported by the XLSX format, *ObjTables* can only encode limited schema information into spreadsheets.

To help make spreadsheets easy to understand, *ObjTables* also embeds descriptions of each attribute into notes on their column headings. These notes serve as inline documentation for the schema for the dataset.

#### 1.3.5. Enhancing the human-readability of spreadsheets

To make column headings easy to read, *ObjTables* bolds, shades, and freezes the header row(s) of each worksheet.

### 1.4. Format for schemas for structured, human-readable spreadsheets

*ObjTables* represents datasets as attribute graphs, or graphs of typed objects, where each object and its attributes are represented by a node and each relationship is represented by an edge. For example, the dataset of genes and transcripts in Fig. 1 of the main text is composed of instances of three classes (genes, transcripts, and locations) which are linked via three relationships (between transcripts and genes, genes and locations, and transcripts and genes) and which have several attributes (gene and transcript ids, gene symbols, and 3' and 5' coordinates). More detailed documentation is available at https://objtables.org.

*ObjTables* provides a simple tabular format for describing the classes that comprise a dataset; the relationships between the classes; the attributes of the classes; and how the classes, relationships, and attributes are encoded into worksheets, rows, and columns. Schema tables contain one row for each class, relationship, and attribute, and have four required and additional optional columns. Fig. 1b of the main text shows an example schema for datasets of genes and their splice variants.

#### 1.4.1. Classes

The name of each class and the title of the corresponding worksheet are defined via the `!Name` column. Each name must begin with a letter and be composed of letters, numbers, and underscores. The `!Type` column indicates whether each row defines a class (value of `Class`) or relationship or attribute (value of `Attribute`). The `!Parent` column can indicate the superclass of each class. Subclasses inherit their parents' relationships and attributes. The `!Format` column indicates how each class is encoded into spreadsheets; the value `row` indicates that the class is encoded into its own worksheet, the value `multiple_cells` indicates that the class is encoded into groups of columns in the corresponding worksheets for its related classes, and the value `cell` indicates that the class is encoded into a single column in the corresponding worksheets for its related classes using a grammar. The optional `!Verbose name` column can define a more human-readable title for the corresponding worksheet or column heading of each class.

#### 1.4.2. Relationships and attributes

The name of each relationship and attribute and the heading of the corresponding column is defined via the `!Name` column. Similar to classes, names must begin with letters and can only include letters, numbers, and underscores. The `!Type` column indicates whether each row defines a class (value of `Class`) or relationship or attribute (value of `Attribute`). The `!Parent` column indicates the parent class of each relationship and attribute. The `!Format` column indicates the type of each

relationship and attribute and constraints on their values. The `!Format` column can also indicate the primary attribute of each class, which can be used to encode relationships between objects into spreadsheets. The optional `!Verbose name` column can define more human-readable column headings.

*ObjTables* support four types of relationships: one-to-one (indicated by the format `OneToOne`), one-to-many (`OneToMany`), many-to-one (`ManyToOne`), and many-to-many (`ManyToMany`). Relationship formats have two required arguments. The first argument must indicate the related class. The `related_name` keyword argument must define the name of the reverse direction of the relationship from the related class to the primary class. The *ObjTables* Python package uses this argument to automatically add an attribute to the related class to represent the connected primary objects. These auto-generated attributes make it easy for users to treat the two directions of each relationship symmetrically. For example, the auto-generated attributes enable users to use the same syntax to set and traverse relationships in both the forward and reverse directions.

To support scientific data, *ObjTables* provides a broad range of types of attributes. This includes attributes for Booleans; integers; floats; strings; dates; times; local files and URLs; emails; arrays; data frames; symbolic mathematical expressions; chemical structures and formulae; DNA, RNA, and protein sequences; and sequence features and motifs. To help researchers annotate scientific data, *ObjTables* also provides attributes for the identifiers of entries in databases, terms in ontologies, units, and uncertainties. For example, researchers could use the attribute type for identifiers to use ChEBI[6] identifiers to describe the metabolites observed in a metabolomics experiment or use the attribute type for ontology terms to use Cell Ontology[7] terms to describe the cell type observed in each experiment.

Researchers can specify constraints on the values of attributes through optional keyword arguments. For example, the integer attribute type supports two optional arguments, `min` and `max`, that can indicate the minimum and maximum valid value of an attribute. More information about the supported attributes and constraints is available at https://objtables.org/docs.

## 1.5. Tools for systematically controlling the quality of data in spreadsheets

To help researchers quality control spreadsheets, the *ObjTables* software can use schemas to validate datasets systematically. The software supports five levels of validation. First, *ObjTables* validates that a spreadsheet uses the *ObjTables* layout conventions and markup syntax. Second, *ObjTables* checks that the value of each attribute of each object is consistent with the constraints defined in the schema. For example, *ObjTables* can check that each metabolite has an integer-valued charge and check that each gene has positive 5' and 3' coordinates. Third, *ObjTables* checks that each relationship encoded using a primary attribute can be decoded. For example, *ObjTables* can check that the gene that codes for each transcript is defined. Fourth, *ObjTables* checks that the values of each primary attribute are unique. For example, *ObjTables* can check that each gene and transcript has a unique id. Fifth, researchers can use the *ObjTables* Python package to define more holistic validations of entire objects and datasets. For example, researchers can validate that chemical reactions are element-balanced, validate that a chemical reaction network is consistent with thermodynamics and the principle of detailed balance,[8] or validate that a pedigree chart is acyclic. More detailed documentation is available at https://objtables.org.

### 1.6. Programmatically creating, querying, editing and analyzing spreadsheets

To help researchers work with spreadsheets programmatically, the *ObjTables* Python package can generate high-level data structures and methods for working with the datasets of a schema. (a) The Python package can generate Python classes for representing the datasets of a schema. (b) Researchers can use the methods of these classes to create instances of the classes, get and set their properties, link them to other objects, and find objects within datasets. The Python package can also import and export instances of these classes to and from spreadsheet files. (c) These classes make it easy to use Python to analyze datasets. More detailed documentation is available at https://objtables.org.

### 1.7. Comparing the content of spreadsheets

To help researchers compare datasets that are encoded in the same schema, the *ObjTables* software can use schemas to determine whether two datasets contain the same content and identify their differences. *ObjTables* determines whether two datasets are equivalent by encoding the datasets into attribute graphs, aligning their graph representations, and identifying the differences in the nodes, edges, and attributes of these representations. As described above, *ObjTables* encodes datasets into graphs by representing each object and its attributes as a node and representing each relationship as an edge. This approach ignores the order of the objects, relationships, and attributes within datasets (e.g., orders of worksheets, rows, and columns), which is often not semantically meaningful. For example, a researcher could use this to compare two reconstructions of the metabolic network of the same organism published by two different researchers. More detailed documentation is available at https://objtables.org.

### 1.8. Merging and splitting spreadsheets

To help researchers integrate data, the *ObjTables* software can automatically merge and split datasets that are encoded in the same schema. The software can merge datasets by representing datasets as graphs, aligning their nodes and edges, and taking the union of their edges. For example, a researcher could use this to merge separate datasets of intracellular metabolite concentrations, the reactants and products of metabolic reactions, and the kinetic rates of metabolic reactions into a single multi-dimensional dataset.

Conversely, the software can split a dataset by representing it as a graph, cutting a specified set of edges, and collecting the resulting connected subgraphs. For example, this could help a researcher analyze a specific intracellular pathway within a large dataset of multiple pathways by extracting the information about that pathway from the dataset.

More detailed documentation is available at https://objtables.org.

### 1.9. Revisioning and migrating spreadsheets

Complex datasets and their schemas are often developed over time as researchers gather more information and more types of data become available. *ObjTables* provides two features to help researchers develop datasets iteratively and collaboratively. First, the *ObjTables* software can help researchers track and manage historical versions of datasets by exporting datasets to CSV or TSV files, committing changes to a version control system such as Git, and merging or identifying conflicts between versions of datasets. Together, this can help a team of researchers work

together to develop a dataset. Second, the *ObjTables* software can help researchers revise a schema and update datasets encoded into the schema by exporting the schema to CSV or TSV file, committing the schema to a version control system, and applying the changes to the schema (e.g., adding, removing, and renaming classes and attributes) to the datasets encoded into the schema. This feature can help researchers in emerging scientific fields develop schemas iteratively as new methodologies and information arise. More detailed documentation is available at https://objtables.org.

### 1.10. Converting spreadsheets to and from alternative formats

In addition to XLSX, the *ObjTables* software can encode and decode datasets into and out of the comma- and tab-separated values (CSV and TSV), JavaScript Object Notation (JSON), and YAML Ain't Markup Language (YAML) formats. We recommend using XLSX for viewing, editing, and sharing datasets. We recommend using JSON for importing datasets into programming languages for further analysis. We recommend using CSV or TSV for revisioning datasets because they are the most compatible with version control systems such as Git.

### 1.11. Visualizing the structure of a spreadsheet

To help researchers understand data, the *ObjTables* software can generate UML diagrams for schemas.

### 1.12. User interfaces

The *ObjTables* toolkit provides four interfaces: a web application, a command-line program, a web service, and a Python library. The web application, command-line program, and web service provide the core features described above for validating, comparing, pretty-printing, and converting datasets and visualizing schemas. In addition to these core features, researchers can use the Python package to implement attributes for additional types; customize how objects and entire datasets are validated; merge and split datasets; revision schemas and datasets; migrate datasets between versions of their schemas; and programmatically construct, edit, query, and analyze datasets. More information about all four interface is available at https://objtables.org/docs.

## 2. Implementation and testing of *ObjTables*

We implemented the *ObjTables* software tools in Python. We implemented reading and writing CSV, TSV, XLSX, and YAML files with OpenPyXL, pyexcel, PyYAML, and XlsxWriter. We used Lark to implement support for grammars. We implemented the mathematics, science, chemistry, and biology attributes using the Biopython,[9] BpForms,[10] BcForms,[10] NumPy, Open Babel,[11] Pint, Pronto, SymPy,[12] and Uncertainties packages. We implemented the revisioning and migration features using GitPython. We implemented the schema visualization feature using GraphViz. We implemented the web application, command-line program, and web service using Zurb Foundation, cement, and Flask-RESTPlus, respectively.

We used unittest to implement extensive unit tests of the *ObjTables* software with over 98% coverage. Furthermore, we used CircleCI and pytest to execute the tests each time we revised the *ObjTables* source code. We assessed the line coverage of the tests using coverage and Coveralls.

# 3. Case studies of using *ObjTables* to structure, debug, reuse, and compose data

Through making it easier to structure spreadsheets, we believe that *ObjTables* can advance a wide range of research. As an example, we illustrate how *ObjTables* can be used to quality control and integrate information about the kinetics and thermodynamics of *Escherichia coli* metabolism into a comprehensive model. As a second example, we illustrate how we have used *ObjTables* to build a format describing for whole-cell (WC) models. While these tasks could be conducted manually or with custom codes, *ObjTables* makes these tasks easier and more accessible to a wider range of investigators.

The spreadsheets for the case studies are available in CSV, TSV, JSON, XLSX, and YAML formats at https://objtables.org/docs. https://objtables.org/docs also contains several additional example datasets and schemas.

## 3.1. Toward an integrated kinetic-thermodynamic genome-scale model of *Escherichia coli* metabolism

Although metabolism is one of the best-characterized cellular subsystems, we still have limited abilities to predict metabolic phenotypes, such as growth, across genotypes and environments. One of the most promising methods for predicting metabolic phenotypes from genotypes is Flux-Balance Analysis (FBA).[13] However, FBA has limited abilities to make quantitatively accurate predictions due limited quantitative flux constraints. Over the past two decades, researchers have explored a variety of strategies for improving FBA models by incorporating additional constraints based on information such as gene regulation,[14] signal transduction,[15] enzyme abundances,[16,17] reaction kinetic parameters,[18] and reaction thermodynamics.[19]

Enhanced FBA models such as FBAwmc[16] require data about the apparent catalytic velocity, $k_{\text{app}}$, of each enzyme for each reaction. Because these apparent velocities are often not available, investigators often approximate their values as their upper bound, the maximum catalytic rate, $k_{\text{cat}}$, of each enzyme for each reaction, which is achieved at limiting substrate concentrations and vanishing product concentrations. However, living cells rarely achieve these maximum rates under physiological conditions.

One way to create more accurate models is to use tighter upper bounds for $k_{\text{app}}$. Noor et al. have shown that a tighter upper bound for $k_{\text{app}}$ is $k_{\text{cat}}\left(1 - e^{\Delta G/RT}\right)$, where $\Delta G$ is the Gibbs free energy of the reaction, which depends on the concentration of each substrate and product, $R$ is the ideal gas constant, and $T$ is the temperature.[20] These upper bounds for $k_{\text{app}}$ are significantly tighter than $k_{\text{cat}}$ except when $\Delta G \ll -RT$. These upper bounds for $k_{\text{app}}$ require data about the $k_{\text{cat}}$ and $\Delta G$ of each enzyme for each reaction.

While $k_{\text{cat}}$ and $\Delta G$ data are both available from separate sources, it is difficult to merge this information because this data is often reported via ad hoc spreadsheets. One reason why it is difficult to merge reaction data from multiple sources is that reactions are typically described as chemical equations, and reactions can be described by multiple equations. For example, reversible reactions can be described in both their forward (e.g., $A \leftrightarrow B$) and reverse (e.g., $B \leftrightarrow A$) directions. Merging reaction data requires algorithms that understand the semantic meaning of reaction equations.

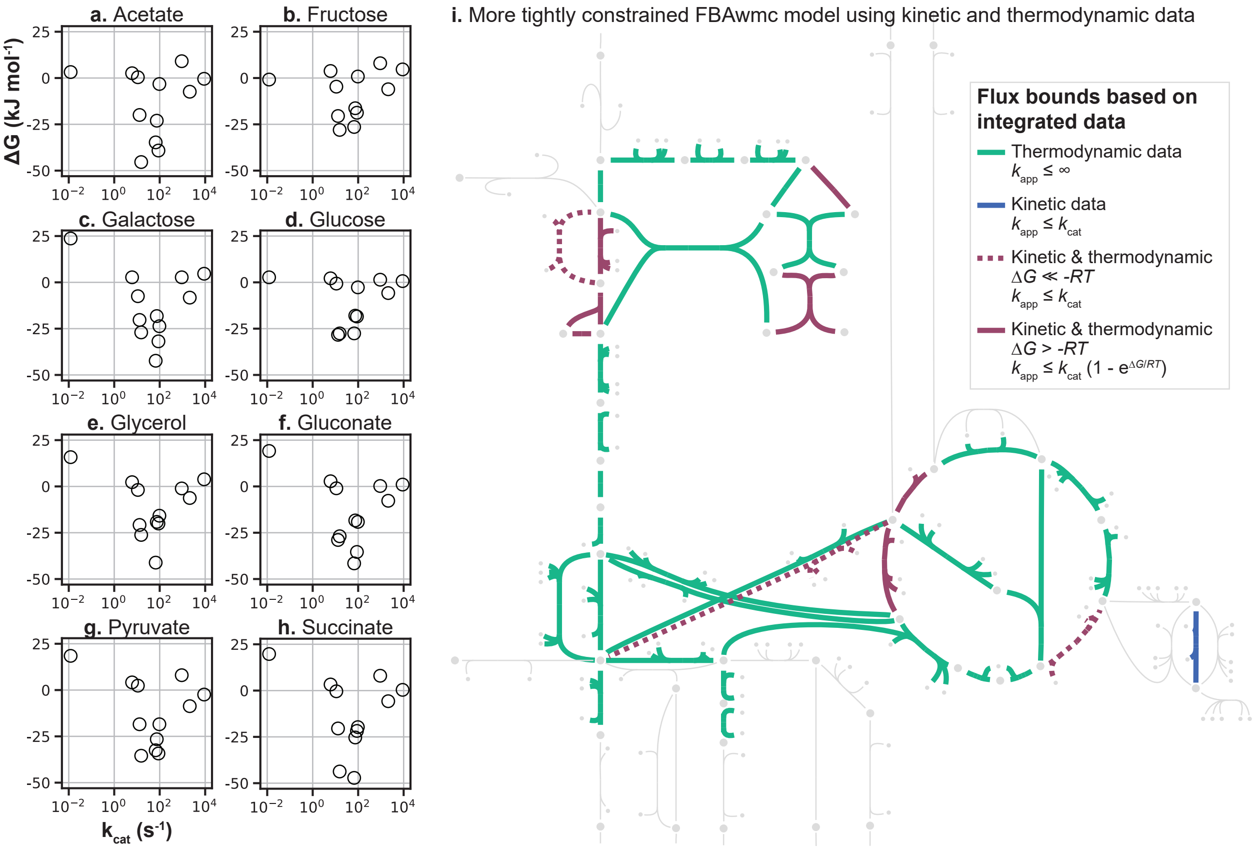


**Figure S1. *ObjTables* can help researchers debug, reuse, and integrate tabular datasets such as supplementary tables to journal articles.** For example, we used *ObjTables* to gather data which could enable an improved FBAwmc model of *E. coli* metabolism. First, we used *ObjTables* to debug $k_{\text{cat}}$ and $\Delta G$ data about *E. coli* metabolic reactions published in ad hoc spreadsheets by Khodayari and Maranas[21] and Gerosa et al.,[22] respectively. Second, we used *ObjTables* to align the $k_{\text{cat}}$ and $\Delta G$ data (**a-h**). Third, we used merged pairs of $k_{\text{cat}}$ and $\Delta G$ data to generate tighter upper bounds for $k_{\text{app}}$ for several reactions (**i**). Finally, the improved $k_{\text{app}}$ bounds could be used to create a better constrained and more predictive FBAwmc model. The spreadsheets for the case study are available in several formats at https://objtables.org/docs.

Toward a more quantitatively predictive model of *E. coli* metabolism, we used *ObjTables* to merge $k_{\text{cat}}$ and $\Delta G$ data for *E. coli* published in ad hoc spreadsheets by Khodayari and Maranas[21] and Gerosa et al.,[22] and use this merged data to generate tighter upper bounds for $k_{\text{app}}$. First, we designed schemas for the spreadsheets that include foreign key constraints between worksheets, grammars for reaction equations, and tab-separated tables embedded into cells in several columns. Second, we used the schemas and the *ObjTables* software to identify and correct errors in the spreadsheets such as swapped column headings, typos in enumerations, syntactically invalid reaction equations, invalid foreign key references, repeated rows, and misaligned columns. Third, we used the *ObjTables* software to automatically identify potentially semantically meaningful differences between the compartments, metabolites, and reactions represented by the Khodayari and Gerosa spreadsheets. Fourth, we manually reviewed the semantic meaning of the differences between the spreadsheets identified by *ObjTables* and manually aligned the datasets. For example, we aligned the identifiers of metabolites that we determined were semantically equivalent, and we aligned the canonical directions of reversible reactions that we determined were semantically equivalent. Once we aligned the datasets, it was trivial to join the datasets by merging pairs of semantically equivalent compartments, metabolites, and reactions. Fig. S1a–h shows the merged

$k_{\text{cat}}$ and $\Delta G$ data. Finally, we used the pairs of merged $k_{\text{cat}}$ and $\Delta G$ data to generate tighter upper bounds for $k_{\text{app}}$, which could enable an improved FBAwmc model of *E. coli* metabolism. Fig. S1i indicates the improved reaction flux constraints in purple.

While we could have merged the $k_{\text{cat}}$ and $\Delta G$ data manually or with custom code, this would have taken significantly more effort. In particular, chemical formula and reaction equations cannot simply be compared by comparing their string representations because their string representations are not unique (e.g., the order of the atoms in a chemical formula has no semantic meaning). Rather, chemical formula and reaction formulae must be compared using algorithms that recognize their semantic meaning such as those implemented by *ObjTables*. In contrast, it only took a few seconds to use the *ObjTables* software to identify the semantically meaningful differences between the Khodayari and Gerosa datasets.

This example illustrates how *ObjTables* can enhance the value of spreadsheets by making it easier to quality control, parse complex spreadsheets, and compose spreadsheets.

## 3.2. Format for composite, multi-algorithmic whole-cell (WC) models

The goal of whole-cell (WC) modeling[23,24] is to develop models that can predict cellular phenotypes from their genotypes and environments. Achieving WC models will likely require a large collaborative effort. One of the most promising ways to build models collaboratively is to combine submodels of separate cellular pathways developed by different researchers.

To properly merge submodels, researchers must verify that the submodels capture the same biology with compatible assumptions, identify and fuse the common species, and remove any redundant reactions. Executing this at the scale required for WC modeling requires structured semantic information about the chemical identity of each species and structured provenance information about the data sources and assumptions behind each submodel.

To facilitate collaboration, we have used *ObjTables* to develop WC-Lang (https://github.com/KarrLab/wc_lang), a format that enables researchers to (a) precisely describe submodels of individual pathways, their semantic meaning, and their provenance and (b) combine submodels into a single multi-algorithmic model. The schema for WC-Lang involves 23 worksheets, 38 classes, 157 relationships, 24 types of attributes, and three grammars (Fig. S2), demonstrating that *ObjTables* can manage large schemas. The schema and examples of models encoded in the schema are available at https://github.com/KarrLab/wc_lang.

We used *ObjTables* to implement WC-Lang for several reasons. (a) *ObjTables* enabled us to create a spreadsheet-based format, which we anticipate will enable modelers to quickly edit thousands of model elements, as well as make it easy for experimentalists to contribute to models. (b) *ObjTables*' graph alignment methods make it easy to merge submodels with minimal code. (c) By providing high-level data structures and methods for manipulating models, *ObjTables* makes it easy to implement multi-algorithmic simulations.

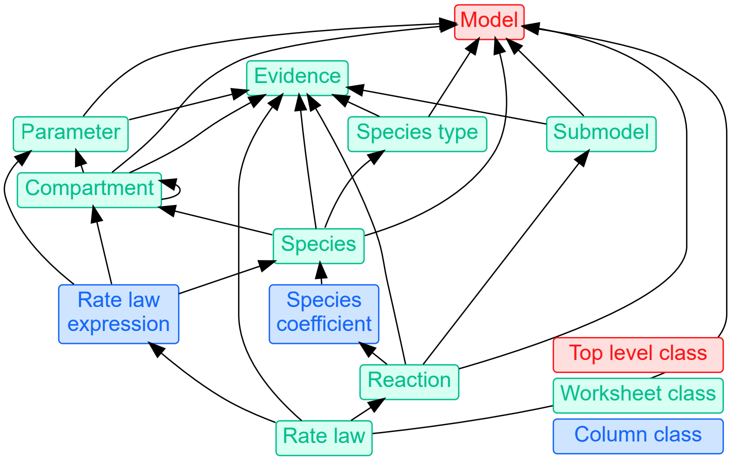


**Figure S2.** ***ObjTables* can help researchers build formats for domain-specific data such as WC-Lang, a spreadsheet format for describing the mathematics, semantics, and provenance of whole-cell models.** WC-Lang involves 23 worksheets, 38 classes, 157 relationships, 24 types of attributes, and three grammars. This diagram indicates the key classes of WC-Lang and their relationships. Red indicates the top-level class that represents models; green indicates classes that map to separate worksheets; blue indicates classes that map to individual columns or groups of columns of spreadsheets for their parent classes. A diagram of the complete schema is available at https://www.objtables.org/docs.

# 4. Comparison of *ObjTables* with other tools

Due to the prevalence of spreadsheets and their limitations, several researchers and companies have tried to develop tools that are both as easy to use and human-readable as spreadsheets, and that can systematically interpret and rigorously validate datasets. This includes other schema systems for spreadsheets, user-friendly interfaces to databases, and hybrid combinations of spreadsheets and databases.

## 4.1. Domain-specific spreadsheet schemas such as IDEOM, ISA-Tab, and MAGE-TAB

Several domains have developed schemas for spreadsheets for specific types of datasets. For example, IDEOM outlines tables for metabolomics data;[25] ISA-Tab outlines tables and columns for capturing experimental studies;[26] and MAGE-TAB outlines tables for capturing microarray data.[27] However, IDEOM, ISA-Tab, and MAGE-TAB are limited to specific domains.

## 4.2. Alternative general-purpose tools for combining spreadsheets with schemas such as SBtab and Table Schema

The above tools help researchers reuse specific dialects of spreadsheets for specific types of datasets. More flexible tools that support custom schemas are needed to help researchers quality control and reuse the complete range of spreadsheets used in science.

Two tools which enable researchers to define custom schemas for spreadsheets are SBtab[3] and Table Schema.[28] SBtab enables researchers to define schemas that describe the objects represented by a spreadsheet and their attributes, use simple markup syntax to indicate the type of object and attribute represented by each worksheet and column, and use simple syntax to describe structured metadata and comments. However, SBtab lacks some of the features that re-

searchers need to create and reuse high-quality spreadsheets. In particular, SBtab only supports a few data types (booleans, numbers, and strings); SBtab does not support relationships; SBtab schemas cannot capture constraints; SBtab does not leverage features of the XLSX format to provide inline help or instant validation; SBtab does not provide software tools for error checking, comparing, and composing spreadsheets; and SBtab cannot translate spreadsheets into object-oriented data structures. *ObjTables* improves upon SBtab by refining SBtab's format for schemas and markup syntax, and combining them with more data types, relationships, an object-relational mapping (ORM) system, and high-level software tools for error checking, comparing, and composing spreadsheets.

Table Schema also enables researchers to create custom schemas for their datasets. However, Table Schema does not support several essential design patterns for human-readability that are common among real-world spreadsheets such as table of contents worksheets, spreadsheet and worksheet-level metadata, additional unstructured worksheets and columns, grouped columns, many-to-many relationships between rows, transposed tables, and embedded grammars. Table Schema also only supports a few data types. Furthermore, Table Schema does include an ORM tool. As a result, it is hard to map datasets encoded into Table Schema into high-level data structures that are easy to analyze with tools such as NumPy, Pandas, scikit-learn,[29] and SciPy in programming languages such as Python. For similar reasons, Table Schema does not provide tools for comparing or composing spreadsheets.

## 4.3. Databases and object-relational mapping (ORM) tools

While relational databases and object-relational mapping (ORM) tools such as MySQL and SQLAlchemy support some of the features of *ObjTables*, we believe that they are too complex for many researchers. In addition, they are less immediately compatible with revisioning and asynchronous collaboration via version control systems such as Git. While low-code databases such as Airtable are easier to use, they do not provide ORM tools for mapping dataset to high-level data structures, and they are not immediately compatible with version control systems such as Git and journal archiving because they provide limited capabilities for exporting and importing datasets to and from files. Some advantages of databases and ORMs over *ObjTables* are that they are more performant, they can handle larger datasets, and there are many existing tools for connecting to databases from a wide range of languages.

## 4.4. Hybrid database-spreadsheet tools such as DataSpread

Another potential way to achieve the features of *ObjTables* is to combine spreadsheet tools with databases. For example, DataSpread[30] links spreadsheets with schemas via relational databases. However, this hybrid approach is cumbersome for users because it requires users to run a database. We believe that this is too complex for use with supplementary datasets to journal articles. Some advantages of this approach over *ObjTables* are that it is more performant and can handle larger datasets.

Via a different approach, Tyszkiewicz[31] and Cunha et al.[32] have explored encoding relational databases into spreadsheets. However, their approaches create cumbersome spreadsheets that mirror the tables of a relational database. These spreadsheets are difficult for humans to read, negating some of the benefits of spreadsheets.

### 4.5. Data serialization formats such as JSON, XML, and YAML

Data serialization formats such as JSON, XML, and YAML are good formats for exchanging information between machines. Some advantages of these formats over *ObjTables* are that they are simpler and easier for machines to parse. In addition, there are many libraries for reading and writing these formats for a wide range of programming languages. However, these formats are not well-suited for supplementary data because they are hard for humans to read and write. Furthermore, many fewer researchers are familiar with these formats than the XLSX format.

## 5. Future directions for *ObjTables*

Realizing the full potential of *ObjTables* as a platform for exchanging, comparing, and composing data will likely require the development of additional capabilities and resources and community adoption of *ObjTables* as a meta-standard for scientific data. Below are brief descriptions of several potential future directions for enhancing *ObjTables*.

### 5.1. Additional types of attributes for additional types of data

We have developed attributes for a wide range of types of data. To better support specific fields of science, the community will need to develop additional types of attributes for additional types of data. For example, a type of attribute for the Human Genome Variation Society's variant nomenclature[5] would make it easier to encode genetic information into spreadsheets, and a type of attribute for geographic coordinates would make it easier to encode geoscience information into spreadsheets. We encourage researchers to contribute additional types of attributes to the *ObjTables* Git repository, and we plan to release new versions of *ObjTables* as we incorporate additional types of attributes.

### 5.2. Additional layouts to make some datasets easier for humans to read

Currently, researchers use a wide range of layouts to encode data into spreadsheets. To make spreadsheets easier to reuse, we believe that the community should focus on a limited number of layout patterns. As a result, *ObjTables* currently supports the most common layout patterns. These layout patterns are sufficient to capture any dataset. Nevertheless, we recognize that some datasets may be more human-readable with other layouts. For example, multi-level headings could make it easier to represent to some types of data. We encourage users to share suggestions for additional layouts by posting issues to the *ObjTables* Git repository.

### 5.3. Libraries for additional programming languages

Currently, the *ObjTables* library is available as a Python package. We selected Python because it is one of the most popular programming languages across many fields of science and engineering. To make it easier for more researchers to use *ObjTables*, we hope to develop additional libraries for other languages such as C/C++, Java, MATLAB, and R.

### 5.4. A registry of schemas to facilitate standardization

Comparing and composing data with *ObjTables* requires authors to use the same schema. To help communities align on schemas for representing the same type of data, we hope to develop

a registry of schemas. The registry would also make *ObjTables* easier to use by enabling researchers to reuse existing schemas. This would reduce the need for researchers to develop their own schemas.

### 5.5. Graphical user interface viewing and edits *ObjTables*-encoded spreadsheets

As described in Section 1.1, we designed *ObjTables* as a complement to the XLSX format so that users could continue to use their favorite spreadsheet program on their favorite operating system (e.g., Microsoft Excel 2013 on Windows 7) as a graphical user interface GUI) for viewing and editing datasets. To integrate schemas into spreadsheets programs as best as possible, *ObjTables* schemas can be described as additional worksheets or separate XLSX files, and *ObjTables* can encode schemas into notes on the heading of each column and validation on each cell. Nevertheless, some users would likely prefer a more direct GUI for *ObjTables*.

One potential way to implement a GUI is as an add-in to Microsoft Excel. However, it would take significant effort to support all of the versions of Excel (e.g., 2000, 2003, 2007). This would be important because only 17% of organizations use the latest version. Furthermore, add-ins for Excel would only benefit Excel users and not users of other programs such as Apple Numbers and LibreOffice Calc.

A second potential way to implement a GUI is as an extension to Google Sheets. However, this would have similar limitations to an Excel add-in, and Google Sheets is slow for large datasets.

A third potential way to implement a GUI is to develop a standalone desktop program or web application. However, this would require significant effort and would likely never match the feature set and performance of Microsoft Excel. Furthermore, many users would likely prefer the familiarity of Excel.

Another potential solution is to implement a GUI just for designing schemas. This could be implemented as a simple web application.

### 5.6. Community adoption of *ObjTables* as a meta-standard for data

Ultimately, realizing the full potential of *ObjTables* as a platform for comparing and composing data will require adoption by the community. This will require addressing the community's needs and teaching the community how to use *ObjTables*. Currently, we encourage the community to provide input through GitHub issues or pull requests. Long-term, we hope other members of the community will join the *ObjTables* team. To encourage the community to use *ObjTables*, we have begun to advertise *ObjTables* through a variety of online registries, online forums, and community mailing lists and develop extensive documentation. Long-term, we also aim to push the community to publish reusable supplementary spreadsheets by encouraging journals and data registries such as Dryad, FigShare, GitHub, and Zenodo to require authors to submit supplementary spreadsheets in a reusable format such as *ObjTables*.

## References


1. Ecma International. Standard ECMA-376: Office Open XML file formats. https://www.ecma-international.org/publications/standards/Ecma-376.htm (2016).

2. International Organization for Standardization. ISO/IEC 29500-1:2016: Information technology – Document description and processing languages — Office Open XML file formats. https://www.iso.org/standard/71691.html (2016).

3. Lubitz, T. *et al.* SBtab: a flexible table format for data exchange in systems biology. *Bioinformatics* **32**, 2559–2561 (2016).

4. International Committee on Standardized Genetic Nomenclature for Mice. Guidelines for Nomenclature of Genes, Genetic Markers, Alleles, and Mutations in Mouse and Rat. http://www.informatics.jax.org/mgihome/nomen/gene.shtml (2018).

5. den Dunnen, J. T. *et al.* HGVS recommendations for the description of sequence variants: 2016 update. *Hum. Mutat.* **37**, 564–569 (2016).

6. Hastings, J. *et al.* ChEBI in 2016: Improved services and an expanding collection of metabolites. *Nucleic Acids Res.* **44**, D1214–D1219 (2016).

7. Diehl, A. D. *et al.* The Cell Ontology 2016: enhanced content, modularization, and ontology interoperability. *J. Biomed. Semantics* **7**, 44 (2016).

8. Ederer, M. & Gilles, E. D. Thermodynamic constraints in kinetic modeling: thermodynamic-kinetic modeling in comparison to other approaches. *Eng. Life Sci.* **8**, 467–476 (2008).

9. Cock, P. J. *et al.* Biopython: freely available Python tools for computational molecular biology and bioinformatics. *Bioinformatics* **25**, 1422–1423 (2009).

10. Lang, P. F. *et al.* BpForms and BcForms: tools for concretely describing non-canonical polymers and complexes to facilitate comprehensive biochemical networks. *Genome Biol.* (Accepted).

11. O'Boyle, N. M. *et al.* Open Babel: an open chemical toolbox. *J. Cheminform.* **3**, 33 (2011).

12. Meurer, A. *et al.* SymPy: symbolic computing in Python. *PeerJ Comput. Sci.* **3**, e103 (2017).

13. Orth, J. D., Thiele, I. & Palsson, B. Ø. What is flux balance analysis? *Nat. Biotechnol.* **28**, 245–248 (2010).

14. Covert, M. W., Schilling, C. H. & Palsson, B. Regulation of gene expression in flux balance models of metabolism. *J. Theor. Biol.* **213**, 73–88 (2001).

15. Covert, M. W., Xiao, N., Chen, T. J. & Karr, J. R. Integrating metabolic, transcriptional regulatory and signal transduction models in escherichia coli. *Bioinformatics* **24**, 2044–2050 (2008).

16. Beg, Q. K. *et al.* Intracellular crowding defines the mode and sequence of substrate uptake by Escherichia coli and constrains its metabolic activity. *Proc. Natl. Acad. Sci. U. S. A.* **104**, 12663–12668 (2007).

17. Adadi, R., Volkmer, B., Milo, R., Heinemann, M. & Shlomi, T. Prediction of microbial growth rate versus biomass yield by a metabolic network with kinetic parameters. *PLoS Comput. Biol.* **8** (2012).

18. Desouki, A. *Algorithms for improving the predictive power of flux balance analysis*. Ph.D. thesis, Universität Paderborn (2016).

19. Hoppe, A., Hoffmann, S. & Holzhütter, H.-G. Including metabolite concentrations into flux balance analysis: thermodynamic realizability as a constraint on flux distributions in metabolic networks. *BMC Syst. Biol.* **1**, 23 (2007).

20. Noor, E., Flamholz, A., Liebermeister, W., Bar-Even, A. & Milo, R. A note on the kinetics of enzyme action: a decomposition that highlights thermodynamic effects. *FEBS Lett.* **587**, 2772–2777 (2013).

21. Khodayari, A. & Maranas, C. D. A genome-scale escherichia coli kinetic metabolic model k-ecoli457 satisfying flux data for multiple mutant strains. *Nat. Commun.* **7**, 1–12 (2016).

22. Gerosa, L. *et al.* Pseudo-transition analysis identifies the key regulators of dynamic metabolic adaptations from steady-state data. *Cell Syst.* **1**, 270–282 (2015).

23. Karr, J. R. *et al.* A whole-cell computational model predicts phenotype from genotype. *Cell* **150**, 389–401 (2012).

24. Goldberg, A. P. *et al.* Emerging whole-cell modeling principles and methods. *Curr. Opin. Biotechnol.* **51**, 97–102 (2018).

25. Creek, D. J., Jankevics, A., Burgess, K. E., Breitling, R. & Barrett, M. P. IDEOM: an Excel interface for analysis of LC–MS-based metabolomics data. *Bioinformatics* **28**, 1048–1049 (2012).

26. Sansone, S.-A. *et al.* The first RSBI (ISA-TAB) workshop: "can a simple format work for complex studies?". *OMICS* **12**, 143–149 (2008).

27. Rayner, T. F. *et al.* A simple spreadsheet-based, MIAME-supportive format for microarray data: MAGE-TAB. *BMC Bioinformatics* **7**, 489 (2006).

28. Fowler, D., Barratt, J. & Walsh, P. Frictionless data: Making research data quality visible. *Int. J. Digital Curation* **12**, 274–285 (2017).

29. Pedregosa, F. *et al.* scikit-learn: machine learning in Python. *J. Mach. Learn. Res.* **12**, 2825–2830 (2011).

30. Bendre, M. *et al.* Dataspread: Unifying databases and spreadsheets. *Proceedings VLDB Endowment* **8**, 2000–2003 (2015).

31. Tyszkiewicz, J. Spreadsheet as a relational database engine. In *Proc. ACM SIGMOD Int. Conf. Management Data*, 195–206 (2010).

32. Cunha, J., Saraiva, J. & Visser, J. From spreadsheets to relational databases and back. In *Proc. ACM SIGPLAN Workshop Partial Evaluation Program Manipulation*, 179–188 (2009).
